# Supplementary material for: BigColor: Colorization using a Generative Color Prior for Natural Images
Source: arXiv:2207.09685 source file (2022-07-20)
Supplement: Supplementary file 1 [file z_supple.tex]

\setcounter{section}{0}

\begin{center}
{\Large \bf Supplemental Document}
\end{center}

\section{Qualitative and Quantitative Comparison}
For qualitative comparison to previous methods, we estimated the color results using official implementations for each method except for ToVivid~\cite{TowardVivid} due to the absence of released code.
Instead of reproducing the method of ToVivid and directly estimating the color image from a grayscale image, we requested and received the colorization results of ToVivid~\cite{TowardVivid} from the author.
For the case of DeOldify, which supports {\it stable} and {\it artistic} versions, we chose the stable version showing better performance on the ImageNet~\cite{ImageNet} validation set.

For clear perceptual comparison, all estimated images require identical resolution.
While the CNN-based colorization methods~\cite{CIC,ChromaGAN,InstColor,Deoldify} used in the comparison free from constraints to image resolution and aspect ratio, Coltran~\cite{ColTran} and ToVivid~\cite{TowardVivid} only enable producing the fixed size output with $256 \times 256$ spatial.
To overcome the constraint, ToVivid adopted a trick that resizes the grayscale image to $256 \times 256$ resolution ignoring the aspect ratio.
However, ColTran was vulnerable to the resizing trick due to their downsampling scheme of $64 \times 64$ low resolution.
As a result, we used the $256 \times 256$ resolution for all qualitative comparisons to compare in a situation where all methods are operable.

In this supplemental document, we provide more qualitative and quantitative comparisons. Specifically, qualitative comparison for general image in ImageNet1K validation set shown in \Figs{\ref{fig:sup_cmp1}~\ref{fig:sup_cmp2}~\ref{fig:sup_cmp3}}, qualitative and quantitative comparison for complex images shown in \Fig{\ref{fig:sup_cplx1}} and \Tbl{\ref{table:sup_cplx_fid_color}}.

\section{Qualitative Examples}
We provide more qualitative examples of BigColor, consisting of multi-modal solutions with random code z shown in \Fig{\ref{fig:sup_multimodal}}, color results before and after Lab fusion shown in \Fig{\ref{fig:sup_rgb_lab}}, uncureated colorization results shown in \Figs{\ref{fig:sub_uncurate3}~\ref{fig:sub_uncurate3}}, and examples with limitations shown in \Fig{\ref{fig:sup_limitation}}.

\section{Architecture Details}
We attempted to find an optimal encoder architecture considering the type of activation functions, sequence of the modules, various normalization schemes.
After thorough architecture search, we amount to the current encoder architecture, resulting in the architecture analogous to the BigGAN generator. 
The non-local layer, an crucial component of the original BigGAN generator, is excluded in our encoder due to no performance improvement experimentally.
Drop-out module slightly improve the qualitative performance.

For the generator, we adopt fine layers of BigGAN initialized with pretrained parameters using ImageNet1K training set with $256 \times 256$ resolution. 
The random-sampled $z$ has a dimension of $68 \times 1$, which is different from the original dimension of 119 x 1, as we only use part of the BigGAN generator.
This one dimensional vector is divided into four parts of $17 \times 1$ resolution, concatenated with class code $c$ and amount to $145 \times 1$ dimension.
See \Fig\ref{fig:sup_architecture_detail}.

\section{Color Enhancement Augmentation}

\kkw{Describe details}

\section{User Study Details}
As shown in \Fig\ref{fig:sup_userstudy_gui}, we use a trap image for all test samples in order to filter the insincere participants in Amazon Mechanical Turk (AMT). The trap image is identical to the grayscale reference image. We excluded the subjects who select the trap image as the best colorization result at least one of the 100 test samples. In this way, we found 167 unfaithful ones from 200 total subjects, amounting to selected 33 participants. To select the 100 grayscale images for the test, we randomly sampled color images from ImageNet1K validation set, applied the grayscale transformation, and estimated the color for gray inputs using target colorization methods. To avoid potential bias from the method order, we shuffled the sequence of color image results for all tests.

%%%%%%%%%%%%%%% TEXT END %%%%%%%%%%%%%%%
\input{figures_supple/cmp}
\input{figures_supple/cplx}
\input{tables_supple/tbl_cplx_fid_color}

\input{figures_supple/multimodal}
\input{figures_supple/rgb_lab}
\input{figures_supple/uncurate}
\input{figures_supple/limitation}

\input{figures_supple/architecture_detail}

% Color Enhancement Augmentation

\input{figures_supple/userstudy_gui}
\input{tables_supple/tbl_userstudy}
