# Supplementary material for: BigColor: Colorization using a Generative Color Prior for Natural Images
Source: arXiv:2207.09685 source file (2022-07-20)
Supplement: Supplementary file 2 [file z_supple_kkang.tex]

\setcounter{section}{0}
\setcounter{figure}{0}
\setcounter{table}{0}

\begin{center}
{\Large \bf BigColor: Colorization using \\ a Generative Color Prior for Natural Images\\ \footnotesize ~ \\\Large-- Supplemental Document --}
\end{center}

In this Supplemental Document, we present additional details, analysis, and results. Specifically, we provide:
\begin{itemize}
    \item Details on the network architecture,
    \item User study details,
    \item Additional discussion on the color enhancement augmentation,
    \item Additional examples of the luminance replacement,
    \item Qualitative and quantitative comparisons,
    \item Additional uncurated examples,
    \item Additional examples of the multi-modal colorization, and 
    \item Additional discussions on the limitations.
\end{itemize}

\section{Details on Network Architecture}
% 그림[]는 우리의 encoder-generator model의 overview를 나타낸다.
% 우리는 최적의 encoder-generator architecture를 찾고자 시도하였다. 
% 먼저 encoder의 설계를 위해, 우리는 다양한 activation function, ~를 search하였으며, which amount to BigGAN의 architecture와 유사한 형태로 ,other than Non local layer. 
% Non-local layer 빠진 이유
% Drop-out module 추가
% For generator, 우리는 BigGAN의 high level layer를 사용 (초기화)
% High level layer를 사용하기 때문에, 기존 BigGAN과 다르게 z의 dimension이 달라짐
\Fig{\ref{fig:sup_architecture_detail}} shows the detailed network architecture of {\MethodName}. %network overview of {\MethodName} and encoder-generator architecture in details. %.  \Fig{\ref{fig:sup_architecture_detail}}(b) and (c) show our encoder and generator architectures. 
%\Fig{\ref{fig:sup_architecture_detail}} shows an overview of our encoder-generator model, and \Fig{\ref{fig:sup_encoder}} and %\Fig{\ref{fig:sup_generator}} represent a ResBlock of encoder and generator, respectively.
We designed our encoder architecture by inverting the original BigGAN generator~\cite{BigGAN}. % with the following changes.
%Specifically, we conduct ablation studies of various layers in the BigGAN including activation functions, sequence of the modules, normalization scheme, non-local layer, and drop-out module. \sh{Did we show all the ablation results in the main paper?} \kkang{이 부분은 사실 architecture search 했다는 내용(어떻게 encoder 구조 만들지, layer는 어떻게 쌓고 activation function은 어떻게 사용할지..)이며 이 부분 역시 모두 encoder에 대한 내용입니다.} \kkw{이 부분에 대해서 첨부된 ablation 결과는 따로 없습니다.}
Specifically, our encoder consists of several ResBlocks, which is designed based on the ResBlock of the generator with a couple of modifications.
Specifically, while the generator of BigGAN has non-local layers in a few ResBlocks, we exclude them from the encoder, and we adopt an additional drop-out layer at the end of each ResBlock for performance improvement.
For the generator, we adopt the network architecture of the fine-scale layers of the BigGAN generator.
% Compared to the ResBlocks of the generator, the ResBlock of the encoder does not have non-local layers, but has an additional drop-out layer for performance improvement.
% Specifically, we exclude non-local layers and add drop-out layers for performance improvements.
% Our generator has the same design with the fine-scale layers of the BigGAN generator~\cite{BigGAN}.
%\kkang{교수님 이 부분은 encoder part에 대한 변경사항이며, generator part는 BigGAN generator와 동일합니다.}
%To find an optimal encoder architecture, we investigated the type of activation functions, sequence of the modules, and various normalization schemes, which amount to the current architecture analogous to the BigGAN~\cite{BigGAN} generator.
%The non-local layer, a crucial component of the original BigGAN generator, is excluded in our encoder due to no performance improvement experimentally.
%The drop-out module is included as it slightly improves the qualitative performance.
We initialize the generator with a pretrained BigGAN model on the ImageNet-1K training set~\cite{ImageNet}.
The random vector $z$ fed to the generator has a dimension of $68$, %$\mathbb{R}^{68\times1}$
which splits into four $17$-dim vectors. % of $\mathbb{R}^{17\times1}$. %unlike to $119$ dimensions of the latent vector of the original BigGAN generator. 
We concatenate each split vector with the class code $c$ of dimension $128$,
resulting in a $145$-dim vector. %\mathbb{R}^{128\times1}$, resulting in a vector of $\mathbb{R}^{145\times1}$ that is injected to the generator. 
%See \Fig{\ref{fig:sup_architecture_detail}}.
Our code will be made public upon the acceptance of the paper.

%The random-sampled $z$ is split into four vectors of $17$ dimension, and each vector is concatenated with class code $c$ amounting to $145 $ dimension.
\input{figures_supple/architecture_detail}
%\input{figures_supple/encoder}
%\input{figures_supple/generator}

% We attempted to find an optimal encoder architecture considering the type of activation functions, sequence of the modules, various normalization schemes.
% After thorough architecture search, we amount to the current encoder architecture, resulting in the architecture analogous to the BigGAN generator. 
% The non-local layer, an crucial component of the original BigGAN generator, is excluded in our encoder due to no performance improvement experimentally.
% Drop-out module slightly improve the qualitative performance.

% For the generator, we adopt fine layers of BigGAN initialized with pretrained parameters using ImageNet1K training set with $256 \times 256$ resolution. 
% The random-sampled $z$ has a dimension of $68 \times 1$, which is different from the original dimension of 119 x 1, as we only use part of the BigGAN generator.
% This one dimensional vector is divided into four parts of $17 \times 1$ resolution, concatenated with class code $c$ and amount to $145 \times 1$ dimension.
% See \Fig\ref{fig:sup_architecture_detail}.

\section{User Study}
We designed an Amazon-Mechanical-Turk interface for our user study as shown in \Fig{\ref{fig:sup_userstudy_gui}}. 
For an input grayscale image, a user should select the most preferred colorization image among the results with different methods.
In total, there are 100 test samples.
We shuffled the order of the results to remove any bias in the sequence. %color image results for all tests.
We also intentionally added the input grayscale image as a trap option in the colorization results for the sanity check of the user study.
%in order to collect experimental data from users who provided valid choices, 
%for the differennt results. The trap image is identical to the grayscale reference image. 
We excluded all the subjects who selected the trap image at least one time.
In this way, we selected 33 valid participants out of 200 total subjects. %, amounting to selected 33 participants.
\Tbl{\ref{table:sup_user_study_detail}} shows the full preference scores of all of the participants and statistics that summarize the user scores.
The results show that the participants generally prefer to the results of \MethodName~over the others.
%, demonstrating the effectiveness of {\MethodName}.

\section{Additional Assessment}
\subsection{Impact of Color Augmentation}
%Our color augmentation strategy slightly alters the colors of the real images in the training set
%Our color augmentation strategy enhances the vividness and semantic correctness of synthesized color images by making th
Our color augmentation strategy enhances the vividness and semantic correctness of synthesized color images by slightly altering the colors in the real images in the training set.
Specifically, our color augmentation strategy boosts the colors in the real images in the training set, which is fed to the discriminator during training, only by a small amount so that it does not introduce unwanted distortion to the color distribution of real images.
On the other hand, it still makes the colors of semantically different regions in the training images more distinguishable during the training phase.
In consequence, it helps the generator learn to synthesize semantically more correct and vivid colors.
In this section, we qualitatively demonstrate the effect of our color augmentation.
For the quantitative evaluation, we refer the readers to Tab.~5 in the main manuscript.

\Fig{\ref{fig:sup_aug_cmp}} shows a qualitative comparison of our color augmentation strategy with two baselines: \Method\ without our augmentation and \MethodName\ with post color processing.
For the post color processing, we apply the same color color-balancing method used in \MethodName\ directly to the output of the generator.
%Note that \MethodName\ applies the color-balancing method only to the real samples fed to the discriminator during the training phase.

The results of \MethodName\ without the color augmentation and with the post color processing (\Fig{\ref{fig:sup_aug_cmp}}(b) and (c)) have similar colors while the the results in (c) are slightly more vivid. This implies that our color augmentation scheme does not change the color distribution of the real images in the training set much.
Also, compared to our results in (d), the results without the color augmentation have less vivid and semantically inaccurate colors, e.g., the dull colors of the bricks and wood on the first and second rows, the red color on the accordion on the fourth row, and the red human face on the last row.
While the post processing slightly boosts the color vividness, its results still have the exactly same artifacts as it is applied at the end of the colorization process.
On the other hand, our results have more vivid and semantically correct colors, showing that our color augmentation scheme helps the generator synthesize more vivid and accurate colors.

% human face in the last row is colorized red by the other methods, while 
% As shown by the results of \MethodName\ with post color processing, our color augmentation scheme slightly alters the colors in input images

% We evaluate the impact of our color augmentation by showing a qualitative comparison. 
% See Tab. 5 of the main manuscript for quantitative evaluation.
% \Fig{\ref{fig:sup_aug_cmp}} shows that our color augmentation improves both naturalness and vividness of synthesized color images compared to two baselines: 
% \MethodName\ without our color augmentation and \MethodName\ with a post color processing. 
% For the post color processing, we apply the same color-balancing method used in \MethodName\ to the output of the generator.
% Note that \MethodName\ applies the color-balancing to the real samples fed to the discriminator. 
% Color augmentation of \MethodName\ enables natural and vivid colorization as shown in \Fig{\ref{fig:sup_aug_cmp}}, specifically the bricks, the wood texture, the dog, and the human faces.

\subsection{Luminance Replacement}
% fig : sup_rgb_lab
\MethodName\ brings the high-frequency spatial details of the input grayscale image via luminance replacement.
%exploit high-frequency details of input image by replacing the luminance of synthesized image with input luminance in the CIELAB color space.
\Fig{\ref{fig:sup_rgb_lab}} shows that the luminance replacement enables us to recover high-frequency spatial details while maintaining the high-quality colors synthesized from our generator. % compares the output of the generator and the result of replacing the luminance as described in \Fig{\ref{fig:ablation_fdim_teaser}} (d) and (e) in the main paper.
%Although the generator output also shows good colorization results, the image detail is greatly improved by replacing luminance.

%N
%Our color augmentation scheme enables not only enhancing vividness of color of each semantic part but also estimating more consistent and correct color, resulting in the better scores on FID~\cite{FID} and classification accuracy, as shown in Tab. 5. in the main paper.
%For instance, as shown in 1st and 2nd columns of \Fig{\ref{fig:sup_aug_cmp}}, our color augmentation scheme successfully enhance the colors of brick and wood textures.
%In addition, it helps to produce more consistent colors as shown in 3rd and 4th columns of \Fig{\ref{fig:sup_aug_cmp}}. While the leg guard of a dog is unnaturally colorized with two color even though it is single object in the case of the non-augmentation model, our full model produces a consistent color. 
%Lastly, it also helps to produce semantically accurate colors as shown in 5th and 6th of \Fig{\ref{fig:sup_aug_cmp}}.
%\kkw{Saturation Histogram 결과가 예상과 다름, trainging dataset에 대해서 시도 예정}

\section{Additional Comparisons}
%\section{Qualitative and Quantitative Comparison}
% 기존 방법 구현 details.
% 그림 설명
%\subsection{Implementation}
%In this section, we first describe the implementation details of the previous methods~\cite{TowardVivid,Deoldify,CIC,ChromaGAN,InstColor,ColTran} and then provide additional qualitative and quantitative comparisons. 
In this section, we provide additional qualitative and quantitative comparisons against recent colorization methods~\cite{TowardVivid,Deoldify,CIC,ChromaGAN,InstColor,ColTran}.
For the previous methods, we used the official codes from the authors except for ToVivid~\cite{TowardVivid}, which does not provide code at the time of our submission.
%We used the official codes for the previous methods except ToVivid~\cite{TowardVivid} which does not provide code at the time of our submission. 
For the results of ToVivid, we requested the authors, and obtained the results for our input images.
%Instead, the authors ToVivid~\cite{TowardVivid} directly provided results for our input images. %which we use directly. %Instead, we directly requested and received the results of ToVivid~\cite{TowardVivid} from the author.
We use the {\it stable} version of DeOldify~\cite{Deoldify}. % which shows better performance on the ImageNet~\cite{ImageNet} validation set.

As ColTran~\cite{ColTran} and ToVivid~\cite{TowardVivid} can only deal with images of a specific size, we conducted our experiments as follows.
For all the other methods except for ColTran and ToVivid, we resized the input images keeping the aspect ratio so that the smaller between the width and height is 256, performed colorization, and cropped the center regions.
Regarding ToVivid, we resized the input images to $256\times256$ ignoring the aspect ratio, obtained their colorization results, and resized the results to recover the original aspect ratios while keeping the smaller between the width and height is still 256. Then, we cropped the center regions of size $256\times256$.
Regarding ConTran, we resized the input images keeping the aspect ratio so that the smaller between the width and height is 256, cropped the center regions of size $256\times256$, and performed colorization.

% We evaluate state-of-the-art colorization methods for the images of resolution $256 \times 256$.
% This is because ColTran~\cite{ColTran} and ToVivid~\cite{TowardVivid} can only deal with the specified resolution. 
% \sh{check this paragraph:}
% %treat the fixed size input image with $256 \times 256$with For fair comparison, all colorized images should have identical spatial resolution. 
% %While the CNN-based colorization methods~\cite{CIC,ChromaGAN,InstColor,Deoldify} are free from the constraints to input resolution and aspect ratio, ColTran~\cite{ColTran} and ToVivid~\cite{TowardVivid} can only treat the fixed size input image with $256 \times 256$ due to their structure.
% To overcome this constraint, ToVivid~\cite{TowardVivid} adopted a trick that resizes the input image to $256 \times 256$ resolution ignoring the aspect ratio. ColTran~\cite{ColTran} resizes and center crops the input image to $256 \times 256$.
% Considering these aspects, in case of the CNN-based colorization methods and our methods, we center crop the colorization results according to ColTran~\cite{ColTran}, and in case of ToVivid~\cite{TowardVivid}, we restores the colorization results to the original aspect ratio and then center crops them.

\subsubsection{Qualitative Comparisons}
We show additional qualitative comparisons in \Fig{\ref{fig:sup_cmp1}}, \Fig{\ref{fig:sup_cmp2}}, and \Fig{\ref{fig:sup_cmp3}}. 
\MethodName\ outperforms all the compared methods for challenging scenes with diverse semantics and structures. % In these comparison, both images of complex structures and images of simple structures are included, and our method shows superior performance in both cases.

\subsubsection{Comparison on Challenging Images}
As described in the main manuscript, we constructed a curated dataset consisting of 100 complex images based on the number of people. %100 challenging image dataset by selecting images with complex structure based on the number of people.
\Fig{\ref{fig:sup_simple_vs_cplx}} shows representative examples of the simple images and complex images with respect to the number of people.
Note that the complex images not only contain many people, but also have higher image complexity.
%shows the thumbnails of the complex dataset and the whole dataset. Note that the curated complex dataset not only contains many people, but also has higher image complexity.  %of complex images compared to simple images. It can be seen that the challenging images not only includes a lot of people, but also images with a complex structure.
\Tbl{\ref{table:sup_cplx_fid_color}} and \Fig{\ref{fig:sup_cplx1}} show quantitative and qualitative comparisons of different colorization methods. 
Again, {\MethodName} achieves state-of-the-art quantitative and qualitative performance.

\section{Additional Results}

\paragraph{Uncurated Examples}
\MethodName\ enables robust colorization for in-the-wild images. 
We show our colorization results on 100 \emph{uncurated} images in \Fig{\ref{fig:sup_uncurate1}} and \Fig{\ref{fig:sup_uncurate2}}.
%See \Fig{\ref{fig:sup_uncurate_cmp}} for the other compared methods that fail on the challenging uncurated scenes.

\subsection{Multi-modal Colorization}
\MethodName\ allows us to synthesize diverse colors for an input grayscale image.
\Fig{\ref{fig:sup_multimodal}} shows additional results of multi-modal colorization by using different random codes $z$. %, {\MethodName} colorize input the grayscale image with a different color that a given class would represent.

\subsection{Limitations}
% fig : sup_limitation
\Fig{\ref{fig:sup_limitation}} shows three failure cases of \MethodName.
First, {\MethodName} may fail to colorize very small regions such as the ear in the first row in the figure. This is because the spatial resolution of extracted feature $f$ is small as $16\times16$. %, meaning that small regions might be overlooked.
Second, {\MethodName} may struggle with complex images that contain objects with significantly different object classes such as toys and human. %In this example, the class of the image is the toy class, which contaminates the hand with toy color. 
%\kkang{추정되는 근본 원인: 이미지의 class는 장난감으로 붉은 색과 같은 color가 많이 포함됨. 이는 손과 같은  경계이면서 애매한 부분에 장난감 color를 칠해버리는 결과를 산출함, 즉 단일 class로 한 이미지가 정의되어서 생성되는 문제...}
Lastly, {\MethodName} may fail to handle input images considerably different from training images. 
%That is, input grayscale images are expected to lie in a similar distribution of training grayscale images.
Old grayscale photographs could fall into such category. Old photographs deviate from the training-data grayscale distribution due to its film sensitivity and chemical development recipes.
 %  with  input grayscale images often fail to estimate proper color on low quality grayscale images.
%This is because deterioration such as blur or noise of the low quality image deviates the image from the learned distribution of {\MethodName}.

% We provide more qualitative examples of BigColor, consisting of multi-modal solutions with random code $z$ shown in \Fig{\ref{fig:sup_multimodal}}, color results before and after Lab fusion shown in \Fig{\ref{fig:sup_rgb_lab}}, uncureated colorization results shown in \Figs{\ref{fig:sup_uncurate1}~\ref{fig:sup_uncurate2}}, and examples with limitations shown in \Fig{\ref{fig:sup_limitation}}.\kkw{Describe detail of limitation}

% As shown in \Fig\ref{fig:sup_userstudy_gui}, we use a trap image for all test samples in order to filter the insincere participants in Amazon Mechanical Turk (AMT). The trap image is identical to the grayscale reference image. We excluded the subjects who select the trap image as the best colorization result at least one of the 100 test samples. In this way, we found 167 unfaithful ones from 200 total subjects, amounting to selected 33 participants. To select the 100 grayscale images for the test, we randomly sampled color images from ImageNet1K validation set, applied the grayscale transformation, and estimated the color for gray inputs using target colorization methods. To avoid potential bias from the method order, we shuffled the sequence of color image results for all tests.

%%%%%%%%%%%%%%% TEXT END %%%%%%%%%%%%%%%

\input{figures_supple/userstudy_gui}
\input{tables_supple/tbl_userstudy}

\input{figures_supple/aug_cmp}
\input{figures_supple/rgb_lab}

\input{figures_supple/cmp}
\input{figures_supple/simple_vs_cplx}
\input{figures_supple/cplx}
\input{tables_supple/tbl_cplx_fid_color}

\input{figures_supple/uncurate}
\input{figures_supple/multimodal}
\input{figures_supple/limitation}
